# Supplementary material for: Proposal of quantum repeater architecture based on Rydberg atom quantum processors
Source: arXiv:2410.12523 source file (2024-10-16)
Supplement: Supplementary file 1 [file Supplementary_Materials.pdf]

# Supplementary Materials: Proposal of quantum repeater architecture based on Rydberg atom quantum processors

Yan-Lei Zhang,[1,2,*] Qing-Xuan Jie,[1,2,*] Ming Li,[1,2,3] Shu-Hao Wu,[1,2] Zhu-Bo Wang,[1,2] Xu-Bo Zou,[1,2,3] Peng-Fei Zhang,[4,5] Gang Li,[4,5,†] Tiancai Zhang,[4,5] Guang-Can Guo,[1,2,3] and Chang-Ling Zou[1,2,3,‡]

[1]*CAS Key Laboratory of Quantum Information, University of Science and Technology of China, Hefei, Anhui 230026, China*
[2]*CAS Center For Excellence in Quantum Information and Quantum Physics, University of Science and Technology of China, Hefei, Anhui 230026, China*
[3]*Hefei National Laboratory, University of Science and Technology of China, Hefei 230088, China*
[4]*State Key Laboratory of Quantum Optics and Quantum Optics Devices, and Institute of Opto-Electronics, Shanxi University, Taiyuan 030006, China*
[5]*Collaborative Innovation Center of Extreme Optics, Shanxi University, Taiyuan 030006, China.*

## I. LONG DISTANCE ENTANGLEMENT

In our model, we need to embody three steps for realizing the quantum repeater. At first, we establish the remote entangment of two atoms by cavity quantum electrodynamics, where the two atoms are placed separately in the cavities connected by a fiber. Secondly, the state swapping between the moving atom and the fixed atom is realized by three C-NOT gates based on the Rydberg interaction. Lastly, the entangled pair with the high fidelity is obtained by entanglement purification, which can be decomposed into single qubit rotations, C-NOT gates and detection operations. By utilizing the remotely entangled atoms with the high fidelity, the entanglement distance can be further extended for the quantum repeater.

### A. Establishing entanglement

An ancilla photon $|A\rangle$ is sent into the cavity $a$ that contains one atom, which is called as the fixed atom. Here we define the polarized photon $|A\rangle \equiv (i|R\rangle + |L\rangle)/\sqrt{2}$ and the orthogonal state $|D\rangle = (i|R\rangle - |L\rangle)/\sqrt{2}i$. The $|L\rangle$ polarized light does not interact with the fixed atom and enters the cavity, which will acquire a $\pi$ phase shift after leaving the cavity. The light in the $|R\rangle$ polarization also acquires the $\pi$ phase shift through the cavity if the atom is in the state $|0\rangle$. When the atom is in the state $|1\rangle$, the $|R\rangle$ polarized light is blocked from entering the cavity and is directly reflected without any further phase shift [1]. That is due to a normal mode splitting for the atom in the coupling state $|1\rangle$, and the corresponding interaction Hamiltonian between the atom and the cavity can be written as $H_{\text{int}}^{a} = g\left(a|e\rangle_a\langle 1| + a^{\dagger}|1\rangle_a\langle e|\right)$, where $g$ is the coupling strength. Based on the cavity quantum electrodynamics, we have the transformation

$$|0\rangle|A\rangle \xrightarrow{H_{\text{int}}^{a}} -\frac{1}{\sqrt{2}}|0\rangle(i|R\rangle + |L\rangle) = -|0\rangle|A\rangle, \tag{1}$$

$$|1\rangle|A\rangle \xrightarrow{H_{\text{int}}^{a}} \frac{1}{\sqrt{2}}|1\rangle(i|R\rangle - |L\rangle) = i|1\rangle|D\rangle, \tag{2}$$

$$|0\rangle|D\rangle \xrightarrow{H_{\text{int}}^{a}} -\frac{1}{\sqrt{2}i}|0\rangle(i|R\rangle - |L\rangle) = -|0\rangle|D\rangle, \tag{3}$$

$$|1\rangle|D\rangle \xrightarrow{H_{\text{int}}^{a}} \frac{1}{\sqrt{2}i}|1\rangle(i|R\rangle + |L\rangle) = -i|1\rangle|A\rangle, \tag{4}$$

which means that we can realize the entanglement between the photon and the cavity $a$. Then, the photon passes through the circulator and fiber to the cavity $b$, and comes out after going through the same process. The entire processes evolve based on the following Hamiltonian

$$\begin{aligned} H_{\text{int}} &= H_{\text{int}}^{a} + H_{\text{int}}^{b} \\ &= g\left(a|e\rangle_a\langle 1| + a^{\dagger}|1\rangle_a\langle e|\right) + g\left(b|e\rangle_b\langle 1| + b^{\dagger}|1\rangle_b\langle e|\right), \end{aligned} \tag{5}$$

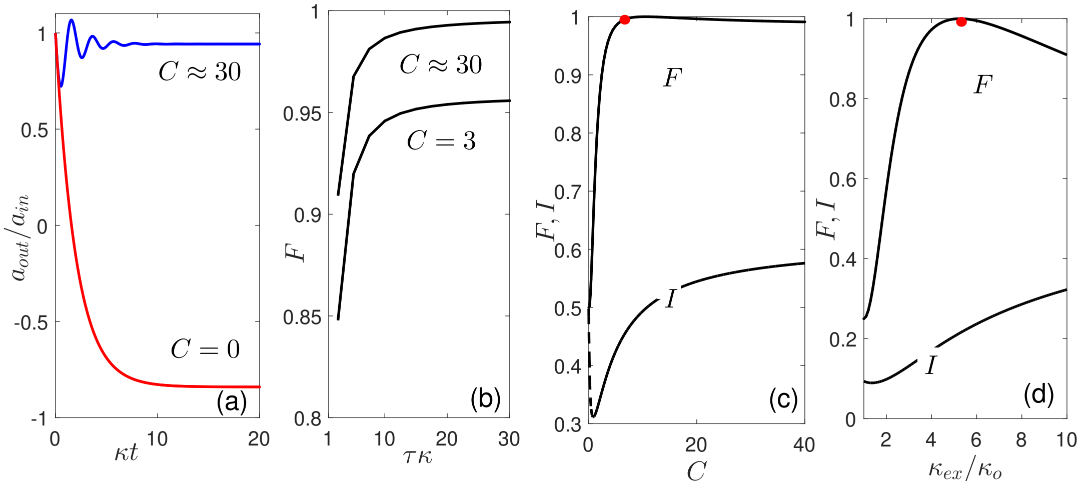


FIG. 1. (a) The dynamical evolution of the output photon, which shows that the time required to reach stability is about $\tau \approx 20/\kappa$, where the parameters are $\kappa_o = 2\pi \times 0.2$ MHz, $\kappa_{ex} = 2\pi \times 2.3$ MHz, $\kappa = \kappa_o + \kappa_{ex} = 2\pi \times 2.5$ MHz, $\gamma = 2\pi \times 3$ MHz, and the cooperativity coupling $C \approx 30$ with the coupling strength $g = 2\pi \times 7.6$ MHz. (b) The fidelity as the input Gaussian pulse length $\tau\kappa$ with the cooperativity $C \approx 30$ and 3. (c) The fidelity $F$ and the efficiency $I$ as the function of the cooperativity $C$ by increasing the coupling strength $g$. (d) The fidelity $F$ and the efficiency $I$ versus the external coupling strength $\kappa_{ex}$ for the weak coupling $g = 2\pi \times 2$ MHz. The red dots are corresponding to the ideal normalized fidelity.

which can be decomposed into segmented evolution. Here we assume that the initial state is $|\psi\rangle_0 = |A\rangle \otimes \frac{1}{\sqrt{2}}(|0\rangle_a + |1\rangle_a) \otimes \frac{1}{\sqrt{2}}(|0\rangle_b + |1\rangle_b)$, and the processes of establishing entanglement can be described as

$$\begin{aligned} |\psi\rangle_0 &\xrightarrow{H^a_{\text{int}}} \frac{1}{\sqrt{2}}(-|A\rangle|0\rangle_a + i|D\rangle|1\rangle_a) \otimes \frac{1}{\sqrt{2}}(|0\rangle_b + |1\rangle_b) \\ &\xrightarrow{H^b_{\text{int}}} \frac{1}{2}(|A\rangle|0\rangle_a|0\rangle_b - i|D\rangle|1\rangle_a|0\rangle_b - i|D\rangle|0\rangle_a|1\rangle_b + |A\rangle|1\rangle_a|1\rangle_b) \\ |\psi\rangle_p &= \frac{1}{2}|A\rangle(|0\rangle_a|0\rangle_b + |1\rangle_a|1\rangle_b) - \frac{i}{2}|D\rangle(|1\rangle_a|0\rangle_b + |0\rangle_a|1\rangle_b), \end{aligned} \tag{6}$$

which clearly shows that we can obtain the Bell state $(|0\rangle_a|0\rangle_b + |1\rangle_a|1\rangle_b)/\sqrt{2}$ or $(|1\rangle_a|0\rangle_b + |0\rangle_a|1\rangle_b)/\sqrt{2}$ if we detect the photon in the state $|A\rangle$ or $|D\rangle$. This is the a post-selection process, which means that we always prepare the maximally entangled state as long as the single photon is detected.

However, the above discussion is the ideal result, and we can prepare the perfect Bell state with the 100% efficiency. In practice, we have to consider the photon loss from the cavity and the imperfect phase shift due to the limited cooperativity $C = 4g^2/(\kappa\gamma)$. The dynamical evolution of the output photon is shown in Fig. 1(a) by the master equation, where we find that the $|a_{out}/a_{in}| < 1$ with the experimental parameters and the duration time $\tau \approx 20/\kappa$ to reach the stability. In addition, the time taken for establishing entanglement also includes the transmission time $l/v$, where $l$ is the length of optical fiber and $v$ is the velocity of light. Therefore, the total time can be written as $T_{\text{esta}}(\approx 20/\kappa + l/v)/P_{\text{succ}}$, where $P_{\text{succ}}$ is the success probability.

To quantitatively illustrate the fidelity, we start with the dynamical equation $da/dt = -\kappa a/2 + \sqrt{\kappa_{ex}} a_{in}$ for the empty cavity under the driving signal $a_{in}$ , where $\kappa_{ex}$ is the external coupling strength and $\kappa$ is the total decay rate, including the $\kappa_{ex}$ and the intrinsic loss $\kappa_o$. The steady state is $a = 2\sqrt{\kappa_{ex}} a_{in}/\kappa$, and the corresponding output signal $a_{out} = a_{in}(\kappa - 2\kappa_{ex})/\kappa$, where $a_{out} = -\sqrt{\kappa_{ex}} a + a_{in}$. When there is the interaction between the atom and the cavity, the dynamical equations are the cavity $da/dt = -\kappa a/2 - ig|1\rangle_a\langle e| + \sqrt{\kappa_{ex}} a_{in}$ and the atom $d|1\rangle_a\langle e|/dt = -\gamma|1\rangle\langle e|/2 - iga|1\rangle_a\langle 1|$. We obtain the steady state $a_{out} = a_{in}(1 + C - 2\kappa_{ex}/\kappa)/(1 + C)$, which depends on the cooperativity $C$. Based on the basic vectors $|L0\rangle$, $|L1\rangle$, $|R0\rangle$, and$|R1\rangle$, the corresponding transformation for the output signal can be written as

$$U_{cz} = \begin{bmatrix} \frac{\kappa_o - \kappa_{ex}}{\kappa_o + \kappa_{ex}} & 0 & 0 & 0 \\ 0 & \frac{\kappa_0 - \kappa_{ex}}{\kappa_o + \kappa_{ex}} & 0 & 0 \\ 0 & 0 & \frac{\kappa_o - \kappa_{ex}}{\kappa_o + \kappa_{ex}} & 0 \\ 0 & 0 & 0 & \frac{1 + C - 2\kappa_{ex}/\kappa}{1 + C} \end{bmatrix}, \tag{7}$$

which is a perfect controlled-Z (CZ) gate if there is no intrinsic loss $\kappa_o = 0$ and the cooperativity is very large $C \gg 1$. The initial

state can be written as a matrix

$$|\psi\rangle_0\langle\psi| = \frac{1}{2}\begin{bmatrix} 1 & -i \\ i & 1 \end{bmatrix} \otimes \begin{bmatrix} \frac{1}{2} & \frac{1}{2} \\ \frac{1}{2} & \frac{1}{2} \end{bmatrix}_a \otimes \begin{bmatrix} \frac{1}{2} & \frac{1}{2} \\ \frac{1}{2} & \frac{1}{2} \end{bmatrix}_b, \tag{8}$$

and the final state can be described by $\rho = U_{cz,b}U_{cz,a}|\psi\rangle_0\langle\psi|U^\dagger_{cz,a}U^\dagger_{cz,b}$. If the CZ gate is perfect, the final gate can be written as $\rho_p = |\psi\rangle_p\langle\psi|$. Therefore, the fidelity can be calculated by $f = \mathrm{tr}(\rho\rho_p)$ and the efficiency is $I = \mathrm{tr}(\rho)$. Based on the measured results, we can further obtain the normalized fidelity $F = f/I$ after the post-seleted measurement. We numerically calculated the relationship between the pulse length and fidelity, and the results are shown in Fig. 1(b), where fidelity gradually reaches the maximum with the increasing of the Guassian pulse length,. When the pulse length is $\tau > 20/\kappa$, and the final fidelity is limited by the cooperativity $C$. In Fig. 1(c), we plot the fidelity $F$ and efficiency $I$ as the function of the cooperativity $C$ in the steady state, which first decreases and then increases by the mumerical calculation. We observe that there is the ideal normalized fidelity, which is labelled by the red dot. In addition, we also notice that we can tune the external coupling $\kappa_{ex}$ to obtain the ideal normalized fidelity even for the weak coupling $g = 2\pi \times 2$ MHz in Fig. 1(d).

In addition to this, measurements of polarization of photon are also likely to be erroneous. Consider a POVM $\mathcal{M}(\rho) = M_A\rho M_A + M_D\rho M_D$, in which $M_{A(D)} = \sqrt{\eta}|A(D)\rangle\langle A(D)| + \sqrt{1-\eta}|D(A)\rangle\langle D(A)|$, with error rate $1-\eta$. To benchmark the result of long distance entanglement, we obtain the specific analytic form

$$F = \frac{(5x^4+8x^3+2x^2+1)+\eta(8x^4-16x^3+8x^2)}{20x^4+8x^2+4}, \tag{9}$$

where

$$x = \frac{\kappa_0-\kappa_{ex}}{\kappa_0+\kappa_{ex}}\frac{1+C}{1+C-2\kappa_{ex}/\kappa}. \tag{10}$$

When there is no error in measurement, that is $\eta = 1$, we have $F = (13x^4-8x^3+10x^2+1)/(20x^4+8x^2+4)$. It is obvious that we have the normalized fidelity $F = 1$ when $x = -1$, which means that $C = (\kappa_{ex}-\kappa_0)/\kappa_0$, and this is also consistent with the numerical results. In practice, the measurement error is taken into account, and the highest fidelity is also obtained when $x = -1$, and the normalized fidelity $F = \eta$, so the fidelity of long distance entanglement is limited by the measurement.

### B. SWAP gate

We establish SWAP gate by combining Rydberg CZ gate and Hadamard gate. In the previous experiment, Rydberg CZ gate is realized by Rydberg blockade, and there is a time-optimal method to get a good pulse [2, 3]. The strong interaction strength $V_{Ry}/2\pi \approx 450$ MHz can be achieved if atoms are placed at 2 $\mu$m separation, and the effective Rabi frequency $\Omega_{eff} = 4.6 \times 2\pi$ MHz can also be achieved. the leading noise source is the decay of Rydberg state, intermediate state scattering, and thermal motion of atoms, and the liouvillian can be written as

$$\frac{d\rho}{dt} = i[\rho, H(t)] + \sum_{l=1}^{N_l}\kappa_l L_l\rho L_l^\dagger - \frac{\kappa_l}{2}\{L_l^\dagger L_l, \rho\}, \tag{11}$$

in which $H(t) = H_0 + H_1(t)$ is the Hamiltonian, in which

$$H_0 = \sum_{j=1,2}\left\{\Delta_e|e\rangle_j\langle e| + \delta_1|1\rangle_j\langle 1| + \delta_r|r\rangle_j\langle r| + [\Omega_{er}|e\rangle_j\langle r| + H.C.]\right\} \tag{12}$$

$$H_1(t) = \sum_{j=1,2}\Omega_{1e}(t)|e\rangle_j\langle 1| + H.C. \tag{13}$$

is the part of Hamiltonian free from control parameters and the control Hamiltonian separately, $L_{a,b,j} = \sqrt{\kappa_{ab}}|b\rangle_j\langle a|$ describe the decay of Rydberg state $|r\rangle$ and intermediate state $|e\rangle$, in which $a = e, r$ and $b = 1, 0, l$, $l$ is the other states in the ground state subspace, $\kappa_{ab} = \kappa_a\mathcal{R}_{ab}$, $\mathcal{R}_{ab}$ is a branching ratio. As the time-optimal Rydberg CZ gate, phase $\theta$ is a optimized parameter, so a single qubit phase gate $U(\theta)$ is needed to realizing a standard CZ gate.

In the level of quantum operations, as the experiment [3], the leading error is dephasing error, and leakage error, so the Kraus operators can be written as

$$K_0 = \sqrt{p_0}X, \tag{14}$$
$$K_1 = \sqrt{p_1}Y, \tag{15}$$
$$K_2 = \sqrt{p_2}Z, \tag{16}$$
$$K_3 = \sqrt{p_3}|l\rangle\langle 1|, \tag{17}$$
$$K_4 = \sqrt{p_4}|r\rangle\langle 1|, \tag{18}$$
$$K_5 = \sqrt{1-p_0-p_1-p_2}|0\rangle\langle 0| + \sqrt{1-p}|1\rangle\langle 1| + |l\rangle\langle l| + |r\rangle\langle r|, \tag{19}$$

$p = \sum_{k=0}^{4} p_k$ is the total error rate for a single qubit, $p_k = \eta_k p$, $\eta_k$ is the percentage of errors, and the quantum channel of a Rydberg CZ gate can be written as

$$\varepsilon_{CZ}(\rho) = \sum_{i,j=0}^{5} U_\theta^\dagger \{K_i \bigotimes K_j [U_{CZ}(\theta)\rho U_{CZ}^\dagger(\theta)] K_i^\dagger \bigotimes K_j^\dagger\} U(\theta) \tag{20}$$

and a CNOT gate can be implemented by two Hadamard gates acting on the target qubit. The high fidelity $F_{cn} \approx 99.5\%$ can be obtained by optimal control, atomic dark states, and atom cooling with the time $\tau < 0.5\ \mu$s, and $\eta_k$ is certificated by experiments. In our numerical simulation, we choose the time-optimal pulse introduced in Ref , we solve the Liouvillian equation to get the phase $\theta \simeq 4.191$, and then choose $p \simeq 0.00365$ to get the same error rate with experiments.

### C. Entanglement Purification

Purification is the distillation of few “perfect” EPR pairs out of many imperfect pairs. A purification protocol that converges faster and involves fewer resources was proposed by Deutsch et al. At the beginning of the whole purification scheme, bilateral random rotations need to be done to get a mixed state that is diagonal under Bell bases, i.e. a Werner state $\rho_W = F|\Psi^-\rangle\langle\Psi^-| + (1-F)/3(|\Phi^+\rangle\langle\phi^+| + |\Phi^-\rangle\langle\Phi^-| + |\Psi^+\rangle\langle\Psi^-|)$, F is the fidelity of initial state. We emphasize that this scheme is a mapping on states that are diagonal in the Bell basis, but need not necessarily be a Werner state form. Generally, we set the initial state as

$$\begin{aligned}\rho_0 &= A\left|\Phi^+\right\rangle\left\langle\Phi^+\right| + B\left|\Phi^-\right\rangle\left\langle\Phi^-\right| + C\left|\psi^+\right\rangle\left\langle\psi^+\right| + D\left|\psi^-\right\rangle\left\langle\psi^-\right| \\ &= \begin{bmatrix} A & & & \\ & B & & \\ & & C & \\ & & & D \end{bmatrix},\end{aligned} \tag{21}$$

where $|\Phi^\pm\rangle = \frac{1}{\sqrt{2}}(|00\rangle \pm |11\rangle)$ and $|\psi^\pm\rangle = \frac{1}{\sqrt{2}}(|01\rangle \pm |10\rangle)$. If we prepare two identical entangled pairs of atoms, as described by $\rho = \rho_0^\alpha \otimes \rho_0^\beta$, where $\alpha$ and $\beta$ represent two nodes respectively. A single qubit rotation $U_\alpha = \frac{1}{\sqrt{2}}I - \frac{i}{\sqrt{2}}\sigma_x$ and $U_\beta = \frac{1}{\sqrt{2}}I + \frac{i}{\sqrt{2}}\sigma_x$ needs to be done respectively for $\alpha$ and $\beta$ node. Then we should do a CNOT gate on qubits in $\alpha$ and $\beta$ node seperately. Results for Rydberg error model have been shown in the main text. In order to show the effects of errors on CNOT gates and detection, here we consider imperfect CNOT gates with depolarizing error, whose error rate equal to $1-p$, and a readout error expressed by a POVM measurement $\mathcal{M}(\rho) = M_0\rho M_0 + M_1\rho M_1$ with a detection accuracy $\eta$, in which $M_1 = \sqrt{\eta}|1\rangle\langle 1| + \sqrt{1-\eta}|0\rangle\langle 0|$ and $M_0 = |r\rangle\langle r| + |f\rangle\langle f| + \sqrt{1-\eta}|1\rangle\langle 1| + \sqrt{\eta}|0\rangle\langle 0|$. After a round of entanglement purification, the analytic result of the reserved entangled pair can be written as

$$\rho = \begin{bmatrix} A' & 0 & 0 & 0 \\ 0 & D' & 0 & 0 \\ 0 & 0 & C' & 0 \\ 0 & 0 & 0 & B' \end{bmatrix}, \tag{22}$$

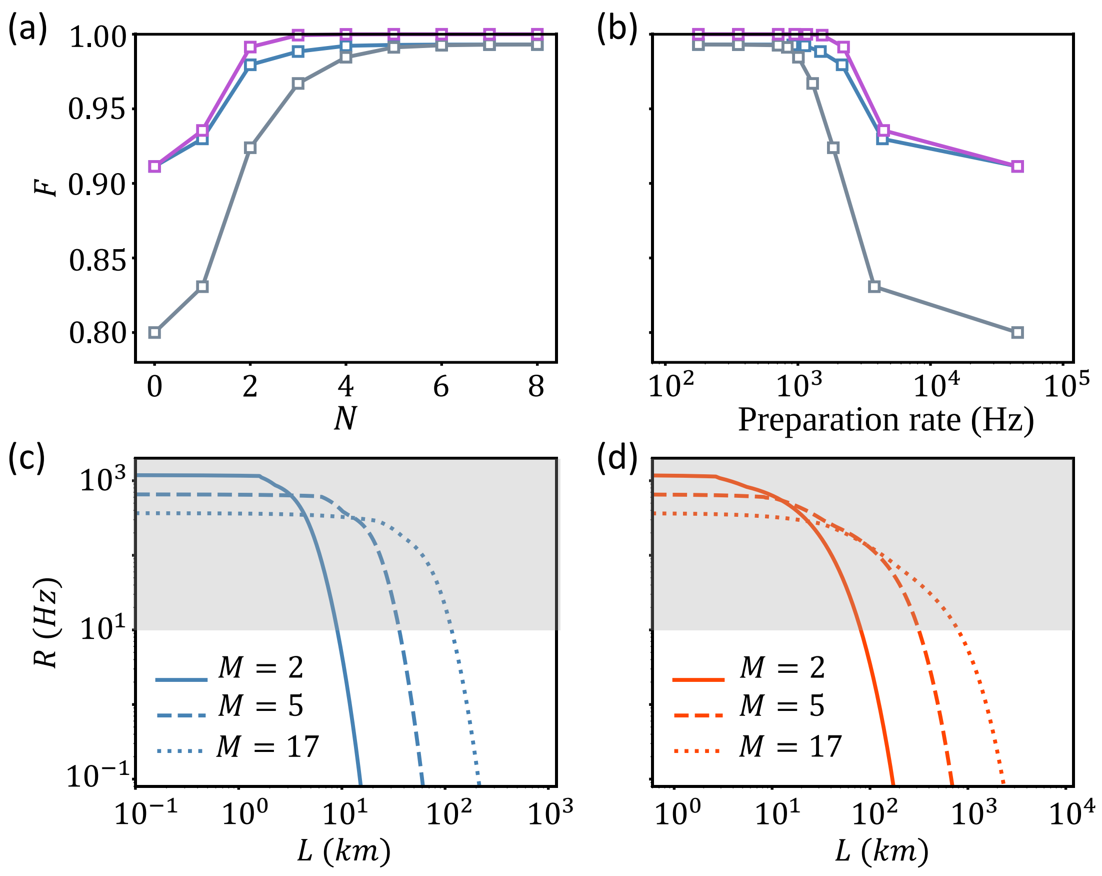


FIG. 2. Results on the depolatization error of CNOT gate and measurement error. (a) e-bit fidelity as a function of the step of purification. Initial fidelity for purple line and blue line is near 0.90, which obtained by experimental parameters, and for gray line is 0.80. The operations for the purple line are ideal, and $F_{CNOT} = 0.995$ and $\eta = 0.99$ for blue line and gray line; (b) e-bit fidelity as a function of e-bit rate, parameters are the same with (a); (c-d) e-bit rate $R$ versus the distance $L$ in the no frequency conversion case (c) and frequency conversion case (d), solid lines, dashed lines and dotted lines are for the $M = 2$, $M = 5$, $M = 17$ separately, points on the line satisfy $F > 0.99$.

and the corresponding parameters can be rewritten as

$$A' = \frac{1}{\Delta}\{p^2(A^2+B^2)[\eta^2+(1-\eta)^2]+2p^2(AC+BD)\eta(1-\eta)+\frac{1-p^2}{8}\}, \tag{23}$$

$$B' = \frac{1}{\Delta}\{2p^2CD[\eta^2+(1-\eta)^2]+2p^2(AD+BC)\eta(1-\eta)+\frac{1-p^2}{8}\}, \tag{24}$$

$$C' = \frac{1}{\Delta}\{p^2(C^2+D^2)[\eta^2+(1-\eta)^2]+2p^2(AC+BD)\eta(1-\eta)+\frac{1-p^2}{8}\}, \tag{25}$$

$$D' = \frac{1}{\Delta}\{2p^2AB[\eta^2+(1-\eta)^2]+2p^2(AD+BC)\eta(1-\eta)+\frac{1-p^2}{8}\}, \tag{26}$$

in which

$$\begin{aligned}\Delta = p^2\{[(A+B)^2+(C+D)^2][\eta^2+(1-\eta)^2] \\ +4\eta(1-\eta)(A+B)(C+D)\}+\frac{1-p^2}{2},\end{aligned} \tag{27}$$

is the probability of success. Here we plot the fidelity as a function of purification steps and preparation rate in Fig. 2(a, b). The trends of each line are similar to the results in the main text. However, the leakage error is contained in the Rydberg error model and atoms are not always in the computational basis, results for the depolarizing channel are slightly better. When the initial state fidelity is $F_0 \approx 0.91$, we need $N \geq 4$ to get a Bell pair with fidelity $F > 0.99$, with the generating rate $R \approx 1.1\,\text{kHz}$, is similar to the case we consider the Rydberg error model. And when the initial state fidelity is $F_0 = 0.8$, only $N \geq 5$ is needed

to get $F > 0.99$, and the effective rate $R \approx 0.8\,\text{kHz}$ is faster than the case we considered in the main text. After many rounds of purification, the final fidelity converges to $F \approx 0.993$, is also better than $F \approx 0.990$ in the main text.

## II. QUANTUM REPEATER

To realize the entanglement at a longer distance, we can realize it by the entanglement swapping. To connect the pairs, we need to perform the Bell measurement on the intermediate node. After entanglement purification, a diagonal state under Bell basis is obtained with form (21), then after a entanglement swapping, the entangled state for two repeaters with longer distance can be expressed as

$$\rho = \begin{bmatrix} \tilde{A} & 0 & 0 & 0 \\ 0 & \tilde{B} & 0 & 0 \\ 0 & 0 & \tilde{C} & 0 \\ 0 & 0 & 0 & \tilde{D} \end{bmatrix}, \tag{28}$$

and the corresponding parameters of state can be written as

$$\begin{aligned}
\tilde{A} =& p\left\{\frac{\eta}{2}\left[(A+B)^2+(C+D)^2\right]+\frac{\eta}{2}(2\eta-1)\left[(A-B)^2+(C-D)^2\right]\right. \\
&\left.+(1-\eta)\left[(A+B)(C+D)+(2\eta-1)(A-B)(C-D)\right]\right\}+\frac{1-p}{4}, \qquad (29)\\
\tilde{B} =& p\left\{\frac{\eta}{2}\left[(A+B)^2+(C+D)^2\right]-\frac{\eta}{2}(2\eta-1)\left[(A-B)^2+(C-D)^2\right]\right. \\
&\left.+(1-\eta)\left[(A+B)(C+D)-(2\eta-1)(A-B)(C-D)\right]\right\}+\frac{1-p}{4}, \qquad (30)\\
\tilde{C} =& p\left\{\frac{1-\eta}{2}\left[(A+B)^2+(C+D)^2\right]+\frac{(1-\eta)(2\eta-1)}{2}\left[(A-B)^2+(C-D)^2\right]\right. \\
&\left.+\eta\left[(A+B)(C+D)+(2\eta-1)(A-B)(C-D)\right]\right\}+\frac{1-p}{4}, \qquad (31)\\
\tilde{D} =& p\left\{\frac{1-\eta}{2}\left[(A+B)^2+(C+D)^2\right]-\frac{(1-\eta)(2\eta-1)}{2}\left[(A-B)^2+(C-D)^2\right]\right. \\
&\left.+\eta\left[(A+B)(C+D)-(2\eta-1)(A-B)(C-D)\right]\right\}+\frac{1-p}{4}, \qquad (32)
\end{aligned}$$

where $\eta$, $p$ appearing in this formula quantify the amount of noise of measurement and C-NOT gate with depolarizing channel. Here we plot the e-bit rate for no frequency conversion case (Fig. 2(c)) and frequency conversion case (Fig. 2(d)), results for Rydberg error models are shown in the main text. The trends of each line are similar to the results in the main text, and the performance under the depolarization channel is still better than Rydberg error model. For $M = 17$ stations, a high fidelity e-bit can be generated at 100 Hz-level until the distance up to 60 km, and high fidelity (0.99) e-bits can be generated at a rate of 10 Hz for $L > 780\,\text{km}$, both are better than the case considered in the main text with 50 km.


* These authors contributed equally.
† gangli@sxu.edu.cn
‡ clzou321@ustc.edu.cn



[1] S. Daiss, S. Langenfeld, S. Welte, E. Distante, P. Thomas, L. Hartung, O. Morin, and G. Rempe, "A quantum-logic gate between distant quantum-network modules," Science **371**, 614 (2021).

[2] S. Jandura and G. Pupillo, "Time-Optimal Two- and Three-Qubit Gates for Rydberg Atoms," Quantum **6**, 712 (2022).

[3] S. J. Evered, D. Bluvstein, M. Kalinowski, S. Ebadi, T. Manovitz, H. Zhou, S. H. Li, A. A. Geim, T. T. Wang, N. Maskara, H. Levine, G. Semeghini, M. Greiner, V. Vuletić, and M. D. Lukin, "High-fidelity parallel entangling gates on a neutral-atom quantum computer," Nature **622**, 268 (2023).
